# Supplementary material for: Charge Transfer Through Redox Molecular Junctions in Non-Equilibrated Solvents
Source: arXiv:2002.06932 source file (2020-02-17)
Supplement: Supplementary file 1 [file SI.pdf]

# Supporting Information to Charge Transfer Through Redox Molecular Junctions in Non-Equilibrated Solvents

Henning Kirchberg,*,† Michael Thorwart,† and Abraham Nitzan*,‡

†*I. Institut für Theoretische Physik, Universität Hamburg, Jungiusstr. 9, 20355 Hamburg, Germany*

‡*Department of Chemistry, University of Pennsylvania, Philadelphia, Pennsylvania 19104, United States of America*

E-mail: henning.kirchberg@physik.uni-hamburg.de; anitzan@sas.upenn.edu

Here we derive (Sec. S1) the solution of the Smoluchowski equation, Eq. (10), for the probability density ($P(x)$) of the reaction coordinate $x$ in the high-damping regime, and (Sec. S2) for the probability density $P(E)$, Eq. (11), in the low-damping regime. Using the resulting probability distribution, we obtain the electron transfer rate in each time segment between the successive electron transfer events, which depend explicitly on the time elapsed since the last transfer event. These rates are used to construct a Monte Carlo procedure (Sec. S3) for sequential one-electron into and out of the molecular bridge, which is used in turn to calculate the average current as well as current-current time correlation functions. In Sec. S4, we derive the electron transfer rate given in Eq. (17) from Eq. (16) in the main text.

# S1 Probability densities in the overdamped regime

The probability densities for the reaction coordinate $x$ are determined by solving the Smoluchowski equation for the overdamped limit ($\gamma \gg \omega_0$). In this limit, the probability densities are velocity independent and satisfy the equation, cf. Eq. (10) of the main text, ($j = A, B$)

$$\begin{aligned} \frac{\partial}{\partial t} P_j(x, t | x'_{TR}, t_{TR}) &= -\frac{\partial}{\partial x}[\dot{x} P_j(x, t | x'_{TR}, t_{TR})] \\ &= \frac{\omega_0}{\hbar\beta\gamma}\frac{\partial}{\partial x}\left[\frac{\partial}{\partial x} + \beta\hbar\omega_0 \frac{d\bar{V}_j(x)}{dx}\right] P_j(x, t | x'_{TR}, t_{TR}) \,, \end{aligned} \tag{S1}$$

where $\beta = \frac{1}{k_B T}$ and $\bar{V}_j = V_j/(\hbar\omega_0)$ with $V_A(x) = \frac{1}{2}\hbar\omega_0 x^2$ and $V_B(x) = \frac{1}{2}\hbar\omega_0 (x-d)^2$.

Eq. S1 should be solved for every time segment between electron transfer events with the initial condition

$$P_j(x, t_{TR} | x'_{TR}, t_{TR}) = \delta(x - x'_{TR}) \ , \tag{S2}$$

where $t_{TR} < t$ is the time of the preceding electron transfer event, given that the event occurred with the reaction coordinate at position $x'_{TR}$. The solution is

$$P_A(x, t | x'_{TR}, t_{TR}) = \sqrt{\frac{D}{2\pi[1 - a^2(t - t_{TR})]}} \exp\left\{-\frac{D}{2}\frac{[x - a(t - t_{TR})x'_{TR}]^2}{1 - a^2(t - t_{TR})}\right\} \ , \tag{S3}$$

$$P_B(x, t | x'_{TR}, t_{TR}) = \sqrt{\frac{D}{2\pi[1 - a^2(t - t_{TR})]}} \exp\left\{-\frac{D}{2}\frac{[x - d - a(t - t_{TR})(x'_{TR} - d)]^2}{1 - a^2(t - t_{TR})}\right\} \ , \tag{S4}$$

where $D = \beta\hbar\omega_0$ and $a(t) = \exp\left[-\frac{\omega_0^2}{\gamma}t\right]$.

# S2 Probability densities in the regime of low damping

In the low-damping limit ($\gamma \ll \omega_0$) phase averaging is fast and the rate is determined by the molecular energy. The corresponding probability distribution obeys a Smoluchowski-type

equation for the energy ($E$) diffusion (cf. Eq. (14.77) in Ref. 1)

$$\frac{\partial P(E)}{\partial t} = \frac{\partial}{\partial E}\left[\gamma \frac{E}{\omega(E)}\left[1 + k_B T \frac{\partial}{\partial E}\right]\omega(E)P(E)\right]. \tag{S5}$$

For a particle moving in a harmonic potential with a constant curvature $\omega_0$ =const., it leads to

$$\begin{aligned}\frac{\partial P(E)}{\partial t} &= \frac{\partial}{\partial E}\left[\gamma E\left[1 + k_B T \frac{\partial}{\partial E}\right]P(E)\right] \\ &= \frac{\partial}{\partial E}\gamma\left[E - k_B T\right]P(E) + \frac{\partial^2}{\partial E^2}\gamma E k_B T P(E).\end{aligned} \tag{S6}$$

The solution may be found by performing a Fourier transform according to $P(c) = \int dE e^{icE} P(E)$, which yields

$$\frac{\partial P(c)}{\partial t} + \left[\gamma c - ic^2 \gamma k_B T\right]\frac{\partial}{\partial c}P(c) = ick_B T\gamma P(c). \tag{S7}$$

It can be solved by using the methods of characteristics $P(c,t) \rightarrow P(c(\tau), t(\tau))$, which implies

$$\frac{\partial P}{\partial \tau} = \frac{\partial P}{\partial c}\frac{\partial c}{\partial \tau} + \frac{\partial P}{\partial t}\frac{\partial t}{\partial \tau}. \tag{S8}$$

Comparison of the coefficients leads to the ordinary differential equations

$$\frac{\partial t}{\partial \tau} = 1 \tag{S9}$$

$$\frac{\partial c}{\partial \tau} = \gamma c - ic^2 \gamma k_B T \tag{S10}$$

$$\frac{\partial P}{\partial \tau} = ick_B T\gamma P(c(\tau), t(\tau)). \tag{S11}$$

Eq. (S9) and Eq. (S10) lead to

$$t = \tau\,, \tag{S12}$$

$$\frac{\partial}{\partial t}\left[\frac{1}{c}\right] + \frac{\gamma}{c} - i\gamma k_B T = 0\,, \tag{S13}$$

and with $1/c \to z$, we find

$$\frac{\partial z}{\partial t} + \gamma z - i\gamma k_B T = 0, \qquad \Rightarrow z(t) = a e^{-\gamma t} + \left(1 - e^{-\gamma t}\right) i k_B T, \tag{S14}$$

while $a$ is determined by the initial condition. Hence, this gives with $c(t=0) = c_0 \Rightarrow a = 1/c_0$

$$c(t) = \frac{1}{a e^{-\gamma t} + (1 - e^{-\gamma t}) i k_B T} = \frac{c_0}{e^{-\gamma t} + (1 - e^{-\gamma t}) i k_B T c_0}\,. \tag{S15}$$

Eq. (S11) then leads to

$$P(t) = A e^{\int_0^t dt' i k_B T c(t')} \tag{S16}$$

$$= A e^{\ln\left(1 - i k_B T c_0 + i k_B T c_0 e^{\gamma t}\right)} \tag{S17}$$

$$= A\left(1 - i k_B T c_0 + i k_B T c_0 e^{\gamma t}\right), \tag{S18}$$

where $A$ may be defined by the initial conditions. With $c_0 = c e^{-\gamma t}/[1 - c i k_B T(1 - e^{-\gamma t})]$, we get

$$P(c,t) = \frac{A}{1 - c i k_B T (1 - e^{-\gamma t})}. \tag{S19}$$

The initial condition $c(t=0) = c_0$ and the fixed initial energy $E_0$ translates to

$$P(c_0, t=0) = \int_{-\infty}^{\infty} dE e^{i c_0 E} \delta(E - E_0) = e^{i c_0 E_0} \equiv A\,. \tag{S20}$$

One now transforms $P(c,t)$ back to $P(E,t)$ and finds

$$P(E,t) = \frac{1}{2\pi}\int_{-\infty}^{\infty} dc \exp\left(-iEc\right) \exp\left[\frac{iE_0 c e^{-\gamma t}}{1 - cik_BT(1-e^{-\gamma t})}\right] \frac{1}{1 - cik_BT(1-e^{-\gamma t})} \tag{S21}$$

$$= \frac{1}{2\pi}\int_{-\infty}^{\infty} dc P(c,t). \tag{S22}$$

We identify $c_p = -i/[k_BT(1-e^{-\gamma t})] = -ih$ as a simple pole and can solve the integral by taking the real axis as contour of integration and an infinite semicircle in the lower half-plane towards the imaginary axis to end up with the residue of the lower half-plane. We have

$$P(E,t) = \frac{1}{2\pi}\oint dc P(c,t) = \lim_{R\to\infty}\int_{-R}^{R} dc P(c,t) + \lim_{R\to\infty}\int_{0}^{\pi} d\theta P(Re^{i\theta}, t) iRe^{i\theta} \tag{S23}$$

$$= \frac{-2\pi i}{2\pi}\mathrm{Res}_{c=-ih} P(c,t), \tag{S24}$$

where one uses $c = Re^{i\theta}$ in the second integral which one can neglect afterwards because $\lim_{|c|\to\infty} P(c,t) \to 0$, if $E \geq 0$. We further rewrite the function $P(c,t)$ as an infinite sum, which leads to

$$P(E,t) = \frac{1}{2\pi}\int_{-\infty}^{\infty} dc \sum_{n=0}^{\infty} \frac{(iE_0 c e^{-\gamma t} - iEc - Ec^2/h)^n (ih)^{n+1}}{n!(ih+c)^{n+1}} \Theta(E) \tag{S25}$$

$$= \frac{1}{2\pi}\int_{-\infty}^{\infty} dc \sum_{n=0}^{\infty} \frac{F(c)^n (ih)^{n+1}}{n!(ih+c)^{n+1}} \Theta(E). \tag{S26}$$

One can use the theorem of residue for each summand, while one has a simple pole at $c = -ih$ of each different power of $n$. This yields

$$P(E,t) = \frac{-2\pi i}{2\pi}\mathrm{Res}_{c=-ih} P(c,t)\Theta(E) = -i\sum_{n=0}^{\infty} \frac{(ih)^{n+1}(\partial^n/\partial c^n) F(c)^n|_{c=-ih}}{n!^2} \Theta(E). \tag{S27}$$

Before calculating each summand, we evaluate the derivatives $(\partial^n/\partial c^n)F(c)$ at $c = -ih$, where we define $(\partial^n/\partial c^n)F(c) = F^{(n)}(c)$.

$$F(-ih) = E_0 h e^{-\gamma t}, \tag{S28}$$

$$F^{(1)}(-ih) = i[E_0 e^{-\gamma t} + E], \tag{S29}$$

$$F^{(2)}(-ih) = -2E/h, \tag{S30}$$

$$F^{(3)}(-ih) = F^{(n)}(-ih) = 0; \text{ for } n \geq 3. \tag{S31}$$

We now evaluate the summands of Eq. (S26) to obtain

$$n = 0 \;\; ih \tag{S32}$$

$$n = 1 \;\; -ih^2[E_0 e^{-\gamma t} + E] \tag{S33}$$

$$n = 2 \;\; ih^3[2![E_0 e^{-\gamma t} + E]^2 + 4EE_0 e^{-\gamma t}]/2!^2 \tag{S34}$$

$$n = 3 \;\; -ih^4[3![E_0 e^{-\gamma t} + E]^3 + 36EE_0 e^{-\gamma t}[E_0 e^{-\gamma t} + E]]/3!^2 \tag{S35}$$

$$n = 4 \;\; ih^5[4![E_0 e^{-\gamma t} + E]^4 + 144EE_0 e^{-\gamma t}[E_0 e^{-\gamma t} + E]^2 + 72E^2 E_0^2 e^{-2\gamma t}]/4!^2 \tag{S36}$$

$$n = 5 \;\; -ih^6[5![E_0 e^{-\gamma t} + E]^5 + 2400EE_0 e^{-\gamma t}[E_0 e^{-\gamma t} + E]^3 + 3600E^2 E_0^2 e^{-2\gamma t}[E_0 e^{-\gamma t} + E]]/5!^2 \tag{S37}$$

...

After some reorganization effort one finds

$$P(E,t) = h \sum_{n=0}^{\infty} \frac{(-h)^n [E_0 e^{-\gamma t} + E]^n}{n!} \cdot \sum_{m=0}^{\infty} \frac{h^{2m} E^m E_0^m e^{-m\gamma t}}{m!^2} \Theta(E) \tag{S38}$$

$$P(E,t) = \frac{1}{k_B T(1 - e^{-\gamma t})} \exp\left[\frac{-(E_0 e^{-\gamma t} + E)}{k_B T(1 - e^{-\gamma t})}\right] \cdot \underbrace{\sum_{m=0}^{\infty} \frac{\left[\frac{EE_0 e^{-\gamma t}}{k_B^2 T^2 (1 - e^{-\gamma t})^2}\right]^m}{m!^2}}_{\text{mod. Bessel func. of 1st kind, zeroth order}} \Theta(E). \tag{S39}$$

We check the normalization by using again $h = 1/[k_B T(1 - e^{-\gamma t})]$,

$$\int_0^\infty dE P(E,t) \stackrel{!}{=} 1 \tag{S40}$$

$$\int_0^\infty dE P(E,t) = h e^{-hE_0 e^{-\gamma t}} \sum_{m=0}^{\infty} \frac{h^{2m} E_0^m e^{-m\gamma t}}{m!^2} \underbrace{\int_0^\infty dE e^{-hE} E^m}_{\frac{m!}{h^{m+1}}} \tag{S41}$$

$$\int_0^\infty dE P(E,t) = e^{-hE_0 e^{-\gamma t}} \sum_{m=0}^{\infty} \frac{(hE_0 e^{-\gamma t})^m}{m!} = 1 \quad \text{q.e.d.} \tag{S42}$$

In the limit $t \to \infty$, we find

$$\lim_{t\to\infty} P(E) = \frac{1}{k_B T} \exp\left(\frac{-E}{k_B T}\right) \Theta(E)\,, \tag{S43}$$

which is the Boltzmann distribution. Moreover, the limit $t \to 0$ corresponds to the limit $h \to \infty$, which yields

$$\lim_{t\to 0} P(E) = \lim_{h\to\infty} P(E) = \sqrt{\frac{1}{2\pi 2h\sqrt{EE_0}}} \cdot e^{2h\sqrt{E_0 E}} \cdot h \cdot e^{-h[E_0+E]}\Theta(E) = \begin{cases} 0 \ \text{ for } \ E \neq E_0. \\ \infty \ \text{ for } \ E = E_0. \end{cases} \tag{S44}$$

$$= \delta(E - E_0)\Theta(E)\,. \tag{S45}$$

The modified Bessel function of the first kind and of zeroth order reads

$$I_0(x) = \sum_{k=0}^{\infty} \frac{(\frac{1}{4}x^2)^k}{k!^2} \tag{S46}$$

$$\lim_{x\to\infty} I_0(x) = \sqrt{\frac{1}{2\pi x}} e^x. \tag{S47}$$

# S3 The numerical procedure

## S3.1 Charge current

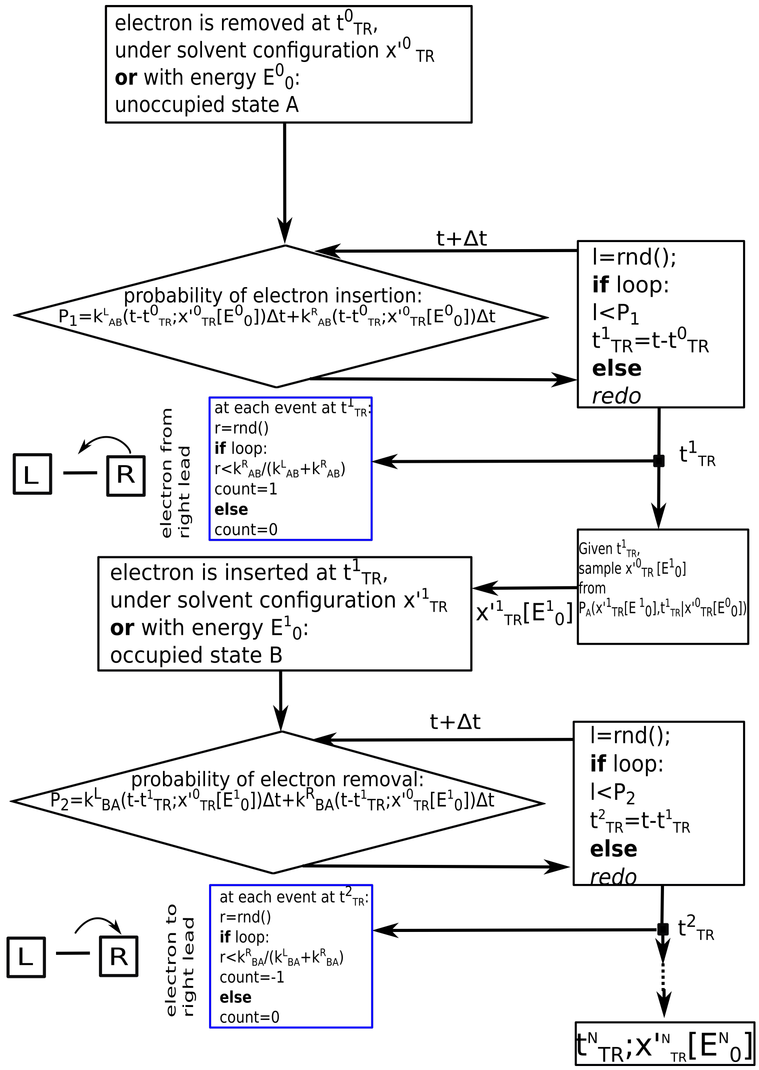


Figure S1: Flow chart of the numerical Monte Carlo algorithm to calculate the charge current.

We calculate the charge current through the molecule by means of a random walk simulation (Monte Carlo) for a sequence of electron insertion (removal) events into (out of) the molecule. The rates for these processes, corresponding to transfer from (to) the left ($K = L$) and right ($K = R$) electrode, are given by Eqs. (14) and (15) of the main text in the overdamped limit, and by Eqs. (19) and (20) of the main text for the low damping

regime, respectively.

The stochastic current is defined as the difference between the sequence of insertion events and the sequence of removal events from and to a given electrode, where each event is represented by the delta-function spike (see Eq. (S48) below). Once an insertion or removal event is recorded at time $t^N_{TR}$, one determines also the electrode involved in this exchange (see Fig. S1). Fig. S2 represents an example of individual electron moves with respect to the right lead. The stochastic current associated with the lead $K$ ($K = L, R$) is then written as

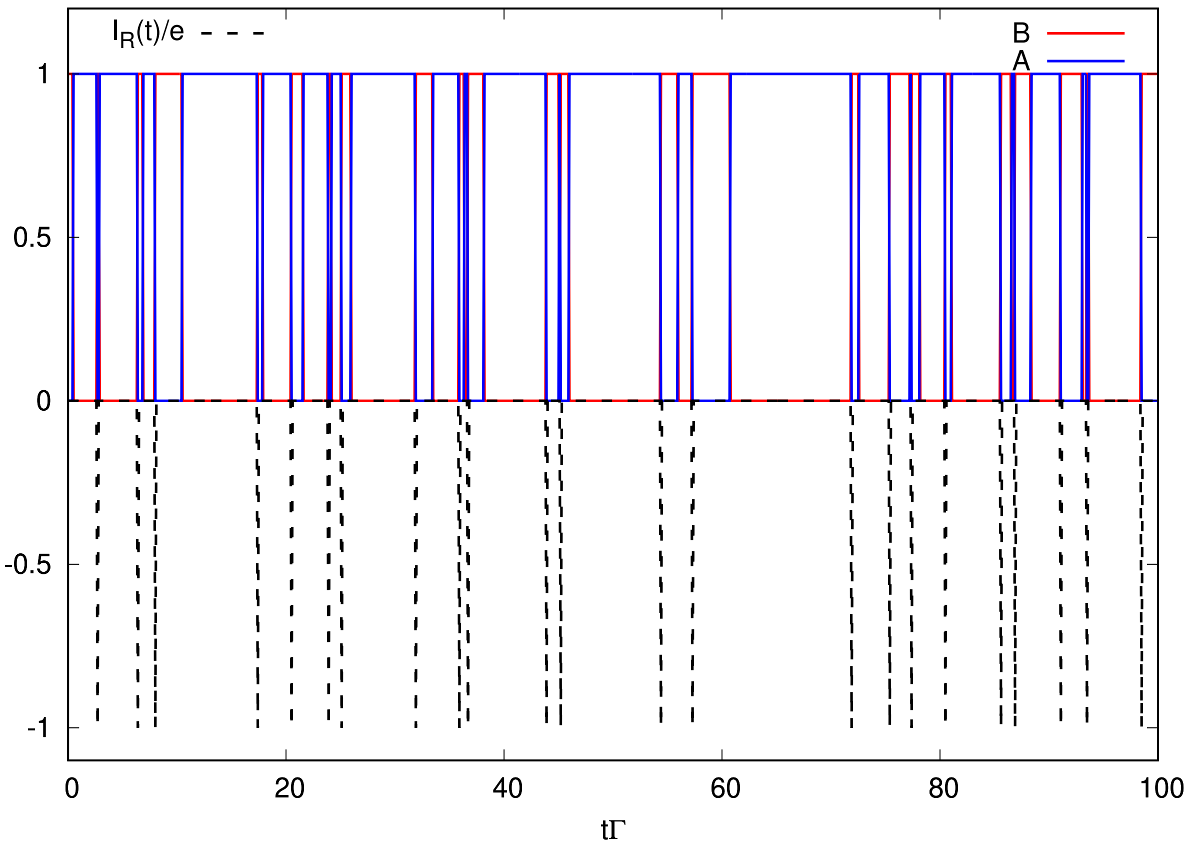


Figure S2: Specific sequence of states $A$ and $B$ at ambient temperature $T = 300K$ for the damping rate $\gamma = 0.001\omega_0$ (overdamped regime for $\gamma \to 0$) and the bias potential of $\Delta\Phi = 300$mV. The electron injection $AB$ from the right lead is recorded by the normalized current $I_R(t)/e$, where $e$ is the electron charge. We set $\mu_R = \mu_L = \Delta E$ (see main text).

$$I_K(t) = e\left[\sum_i \delta(t - t_{Ki}) - \sum_j \delta(t - t_{Kj})\right], \tag{S48}$$

where $e$ is the electron charge and where the first sum goes over all time $t_{Ki}$ at which the electron was inserted in lead $K$, and the second accounts similarly for removal events at times $t_{Kj}$.

The expectation value of the current $\langle I \rangle$ reads

$$\langle I \rangle = \frac{e}{\tau} \int_0^\tau dt \Big[ \sum_i \delta(t - t_i) - \sum_j \delta(t - t_j) \Big] = \frac{e}{\tau}[N - M], \tag{S49}$$

where one observes $N$ electron insertion and $M$ removal processes to a given lead within the time period $\tau$. We assume a steady-state current for the observation window between $(0, \tau)$ for ideally $\tau \to \infty$.

## S3.2 Charge current correlation function

Next, we examine the correlation characteristics of resulting current time-series. The autocorrelation function of the current is defined by

$$C_I(t') = \frac{1}{\tau} \int_0^\tau dt [I(t) - \langle I \rangle][I(t + t') - \langle I \rangle] \,, \tag{S50}$$

where $\tau$ is the time interval of observation. Now, we apply Eqs. (S48) to (S50) to find the autocorrelation of the $\delta$-current pulses as

$$\begin{aligned} C_I(t') = &\frac{e^2}{\tau} \sum_{i;i'} \sum_{j;j'} \int_0^\tau dt \Big[ \delta(t - t_i)\delta(t - t_{i'} + t') - \delta(t - t_i)\delta(t - t_{j'} + t') \\ &- \delta(t - t_j)\delta(t - t_{i'} + t') + \delta(t - t_j)\delta(t - t_{j'} + t') \Big] - \langle I \rangle^2 \\ = &\frac{e^2}{\tau} \sum_{i;i'} \sum_{j;j'} \Big[ \delta(t_i - t_{i'} + t') - \delta(t_i - t_{j'} + t') \\ &- \delta(t_j - t_{i'} + t') + \delta(t_j - t_{j'} + t') \Big] - \langle I \rangle^2 \,. \end{aligned} \tag{S51}$$

We examine the term $I(t)I(t + t')$ as all other terms lead to $-\langle I \rangle^2$.

The current variance is defined by $\sigma_I^2 \equiv C(t'=0)$. In evaluating this term, we use the fact that only $\delta$-functions for $i=i'$ and $j=j'$ remain in $I(t)I(t)$ of Eq. (S51), while all other $\delta$-functions cancel. If we detect $N$ insertion and $M$ removal processes to a given lead, we find

$$\sigma_I^2 = C(t'=0) = \frac{e^2}{\tau}[N+M]\delta(0) - \langle I\rangle^2 = \lim_{\tau'\to 0}\frac{e^2}{\tau\tau'}[N+M] - \langle I\rangle^2 = \langle I^2\rangle - \langle I\rangle^2\,, \quad \text{(S52)}$$

where we replace the $\delta$-function by the inverse of the infinitely small time span $\tau'^{-1}$.

## S4 Derivation of the electron transfer rate Eq. (17) in the main text

We start with the golden rule ET rate given by Eq. (17) in the main text for the $A \to B$ transition

$$k_{AB} = \frac{2\pi}{\hbar} \int_{-\infty}^{\infty} d\epsilon \rho_M(\epsilon) f(\epsilon) \sum_{v;v'} | \langle v | \hat{V}_{A,B} | v' \rangle |^2 \delta(E_A - E_B + \epsilon + E_b(v) - E_b(v')) \,, \qquad \text{(S53)}$$

where $E_A(v)$ and $E_B(v')$ are the eigenvalues of the nuclear (solvent) Hamiltonian (i.e., the harmonic oscillator state on the potential surfaces $E_A(x)$ and $E_B(x)$), $\hat{V}_{AB}$ is the interstate coupling and $\rho_M(\epsilon)$ is the density of single electron states in the metal. We further assume the wide-band limit, i.e., the density of states $\rho_M(\epsilon) = \rho_M =$ const. being independent of the electron energy in the following.

We use the definition of the interstate coupling $\hat{V}_{A,B} = V_{A,B} e^{g(\hat{a}^\dagger - \hat{a})}$ (while $\hat{V}_{A,B}^\dagger = \hat{V}_{B,A}$) according to the spin-boson model after a polaron transformation. Here, $\hat{a}^\dagger$ and $\hat{a}$ are the creation and annihilation operators of the harmonic oscillator state while $g$ describes its coupling strength to the molecular energy states (see Ref.[1] , Chapter 12). Next, we use the identity $\delta(x) = (2\pi\hbar)^{-1} \int_{-\infty}^{\infty} dt e^{ixt/\hbar}$ and write Eq. (S53) in the form

$$\begin{aligned} k_{AB} &= \frac{\rho_M}{\hbar^2} \int_{-\infty}^{\infty} d\epsilon f(\epsilon) \sum_{v;v'} \langle v | \hat{V}_{AB} | v' \rangle \langle v' | \hat{V}_{BA} | v \rangle \int_{-\infty}^{\infty} dt e^{i(E_A - E_B + \epsilon + E_b(v) - E_b(v'))t/\hbar} \qquad \text{(S54)} \\ &= \frac{\rho_M}{\hbar^2} \int_{-\infty}^{\infty} d\epsilon f(\epsilon) \int_{-\infty}^{\infty} dt e^{i(E_A - E_B + \epsilon)t/\hbar} \sum_v \langle v | e^{i\hat{H}_B t/\hbar} \hat{V}_{AB} e^{-i\hat{H}_B t/\hbar} \sum_{v'} | v' \rangle \langle v' | \hat{V}_{BA} | v \rangle \\ &= \frac{\rho_M |V_{A,B}|^2}{\hbar^2} \int_{-\infty}^{\infty} d\epsilon f(\epsilon) \int_{-\infty}^{\infty} dt e^{i(E_A - E_B + \epsilon)t/\hbar} \sum_v \langle v | e^{g(\hat{a}^\dagger e^{i\omega_0 t} - \hat{a} e^{-i\omega_0 t})} e^{g(\hat{a}^\dagger - \hat{a})} | v \rangle \,, \end{aligned}$$

where $\hat{H}_B$ is the Hamilton for the harmonic oscillator, $\omega_0$ is the harmonic mode and $\sum_{v'} |v'\rangle \langle v'|$ is the completeness relation in the oscillator subspace whose orthonormal states obey $\langle v | v' \rangle =$

$\delta_{v,v'}$. We utilize the identity

$$K \equiv \sum_v \langle v| e^{\alpha_1 \hat{a} + \beta_1 \hat{a}^\dagger} e^{\alpha_2 \hat{a} + \beta_2 \hat{a}^\dagger} |v\rangle = e^{(\alpha_1+\alpha_2)(\beta_1+\beta_2)(n+1/2)+(\alpha_1\beta_2-\beta_1\alpha_2)/2}\,, \tag{S55}$$

where $n = \sum_v \langle v| \hat{a}^\dagger \hat{a} |v\rangle$.[1] Since the the oscillator interacts with many solvent degrees of freedom, it exchanges irreversibly energy with the solvent, such that the energy can be defined by $E(t) = n(t)\hbar\omega_0$. Using the definition $n(t) = E(t)/(\hbar\omega_0)$, Eq. (S54) becomes

$$k_{AB} = \Gamma \int_{-\infty}^{\infty} d\epsilon f(\epsilon) \int_{-\infty}^{\infty} dt e^{i(E_A - E_B + \epsilon)t/\hbar - ig^2 \sin(\omega_0 t) + g^2[2n(t)+1][\cos(\omega_0 t) - 1]}\,, \tag{S56}$$

which equals Eq. (17) in the main text after introducing the conditional rate $\Gamma = \frac{\rho_M |V_{A,B}|^2}{\hbar^2}$.

# References

(1) Nitzan, A. Chemical Dynamics in Condensed Phases, Oxford University Press, 2006.
